# Supplementary material for: Mind the Phase: Effective Rank and Representation Health in Legged Locomotion
Source: arXiv:2609.06958 source file (2026-10-15)
Supplement: Supplementary file 1 [file appendix_old.tex]

\section{Additional Background}

\subsection{SimBa Implementation Details}

Our implementation follows the SimBa architecture proposed by~\citet{lee2025simba}, comprising a linear embedding layer, $N$ pre-layer-normalization (Pre-LN) residual blocks, a post-LN, and a linear output head.
Each residual block applies $\mathbf{x} \leftarrow \mathbf{x} + \alpha\,W_2\,\text{ReLU}(W_1\,\text{LayerNorm}(\mathbf{x}))$, where $W_1 \in \mathbb{R}^{4d \times d}$ and $W_2 \in \mathbb{R}^{d \times 4d}$ expand and project the hidden dimension $d$.

The embedding and head weights are initialized orthogonally; residual branch weights use Kaiming normal initialization.
To counteract gradient magnitude growth with depth, each block's residual contribution is scaled by $\alpha = 1/\sqrt{N}$, where $N$ is the number of blocks.
This depth-stable scaling is controlled by a \texttt{depth\_scale} flag and is absent from the original SimBa formulation, which uses $\alpha = 1$.

We provide two integration modes. The first (\texttt{SimbaModel}) subclasses the RSL-RL \texttt{MLPModel} and replaces the internal MLP body (\texttt{self.mlp}) with the SimBa trunk, preserving the full observation-grouping, normalization, and distribution infrastructure of the base class.
The second (\texttt{SimbaActorCritic}) subclasses \texttt{ActorCritic} directly, replacing \texttt{self.actor} and \texttt{self.critic} with separate SimBa trunks of configurable width and depth after the parent \texttt{\_\_init\_\_} has executed; asymmetric sizing is used (actor: $d=256$, $N=1$; critic: $d=512$, $N=2$).
Both variants expose their hyperparameters through drop-in \texttt{@configclass} wrappers (\texttt{RslRlSimbaModelCfg}, \texttt{SpotLocomotionSimbaPPORunnerCfg}) compatible with the Isaac~Lab configuration system.

The original SimBa paper prepends an RMSNorm to the trunk to handle heterogeneous observation scales.
In our integration, this role is filled by RSL-RL's \texttt{empirical\_normalization} flag, which maintains running statistics over observations and normalizes inputs at runtime, making an explicit first-layer RMSNorm redundant.

%===============================================================================
\section{Experiment Details}

\begin{wrapfigure}{r}{0.45\columnwidth}
  \centering
  \vspace{-1em}
  \includegraphics[width=0.40\columnwidth]{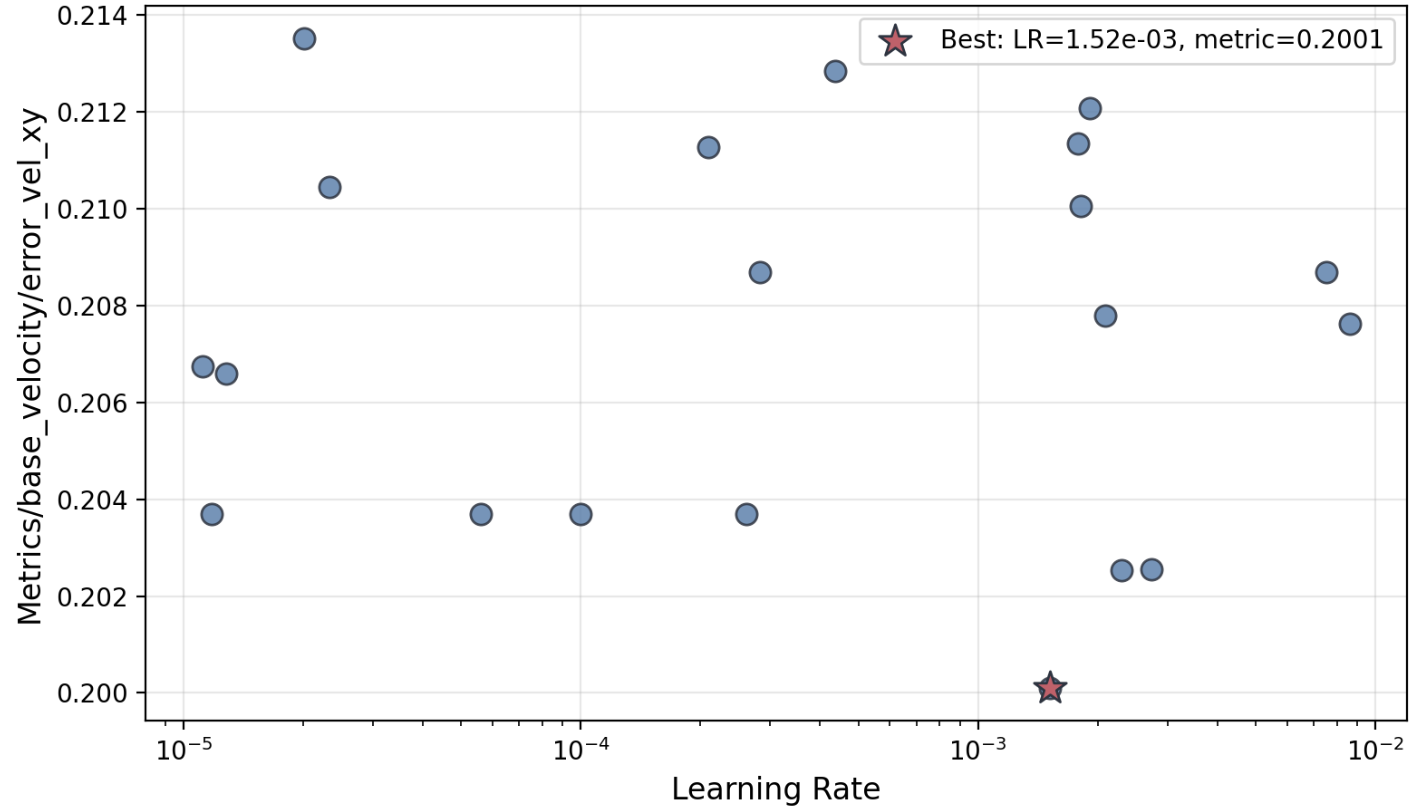}
  \caption{Bayesian optimization search for learning rate on Simba Architecture.}
  \label{fig:sweep}
  \vspace{-1em}
\end{wrapfigure}

\subsection{Code}

We are making all training code open-source, including the infrastructure to run multi-thread IsaacLab across workers used. 

The first version can be found at: \url{https://anonymous.4open.science/r/IsaacLab-F6E2}.

\subsection{Hyper-parameters}

All hyperparameters were set as close as possible to those of the original tasks. For the Spot locomotion environment, we implemented based on the work of \cite{zhu2025versatile}. We varied only the learning rate for Simba, using \(1.5 \times 10^{-3}\). For the MLPs, we used \(1 \times 10^{-3}\) for the three smallest models and \(6 \times 10^{-4}\) for the two largest.

Figure~\ref{fig:sweep} shows the learning rate sweep for Simba, with the top 10 sampled points displayed; in practice, we explored a broader range iteratively.

Both Simba and the MLPs were primarily optimized to maintain healthy representations across multiple depths, as illustrated in Fig.~\ref{fig:mp_simba}.

\begin{figure}[h]
    \centering
    \includegraphics[width=\linewidth]{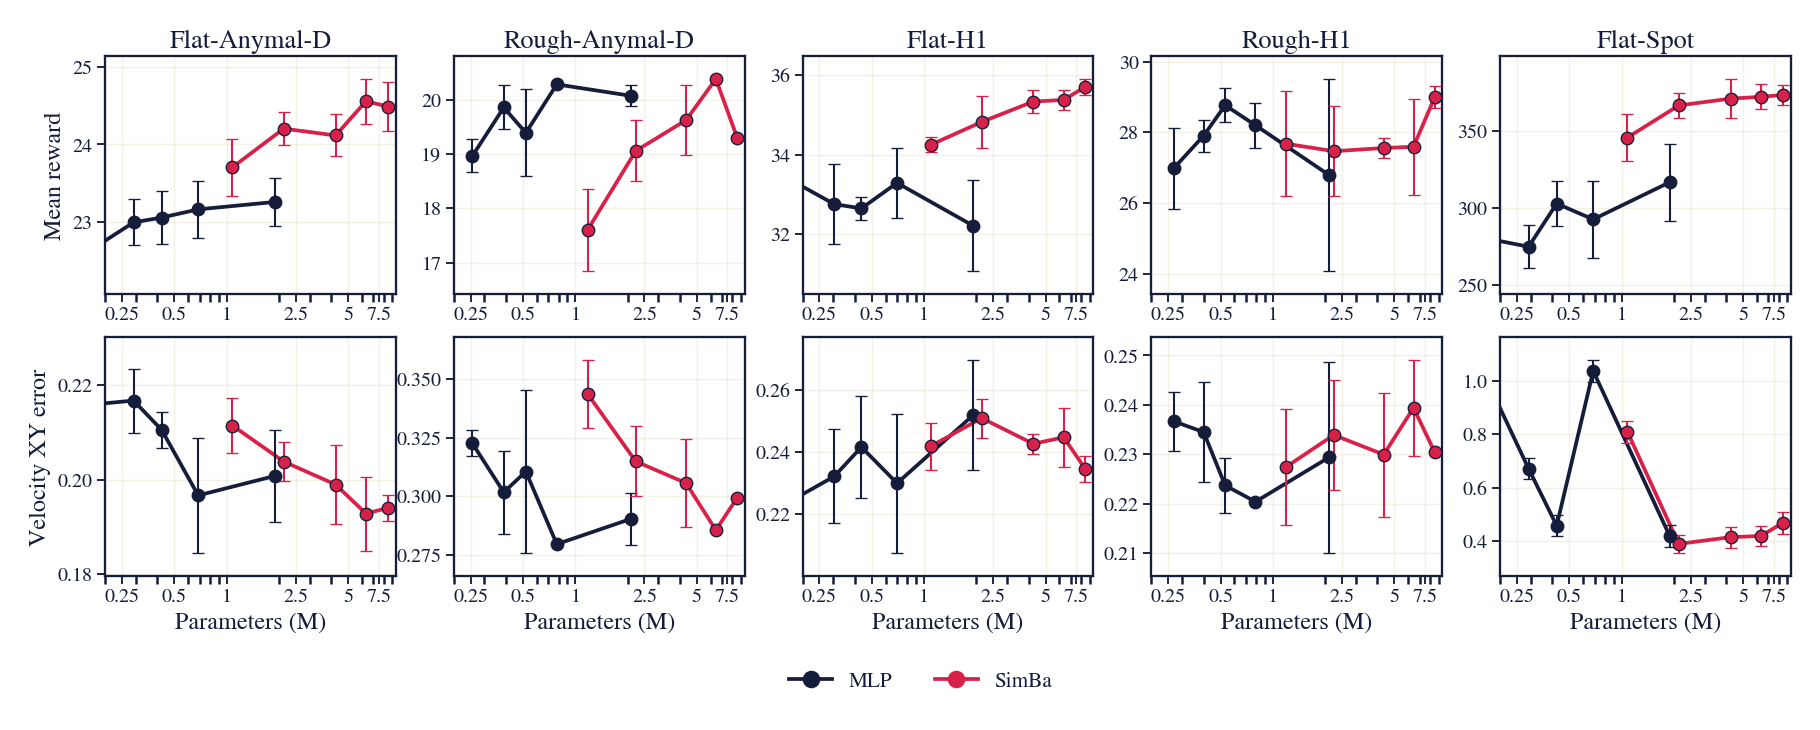}
    \caption{Overall performance across task depths. We compare the classical \textbf{MLP} baseline and \textbf{SimBa} architecture. Markers denote model capacity (parameters, $M$) in logarithmic scale. Both in their actuation range show similar performance, which is the necessary condition for our analysis.}
    \label{fig:mp_simba}
\end{figure}


%===============================================================================
\section{Real-world Experiments}
\label{append:real-word-experiments}

    \subsection{Deployment Details}
    
    \begin{wrapfigure}{r}{0.45\columnwidth}
      \centering
      \vspace{-1em}
      \includegraphics[width=0.45\columnwidth]{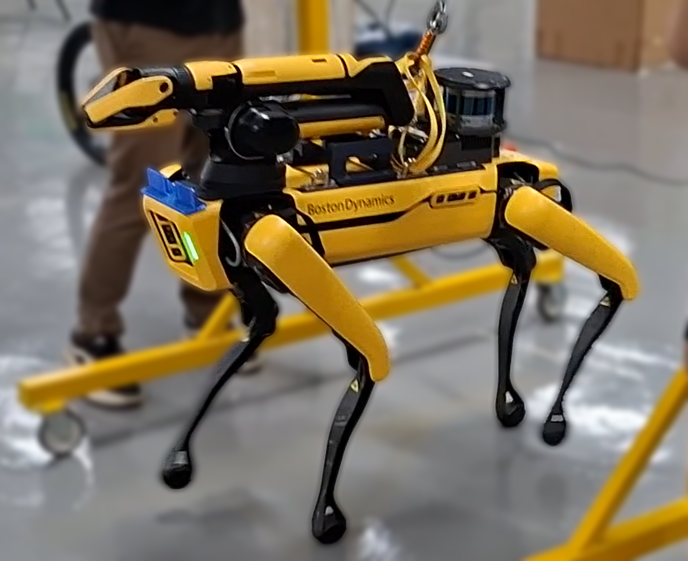}
    \caption{Boston Dynamics Spot used for the real-world experiments.}  \label{fig:exps}
      \vspace{-1em}
    \end{wrapfigure}
    
    We deploy the policy on a Boston Dynamics Spot robot using the ONNX runtime for inference. Robot states are streamed from Spot's proprietary C++ SDK over gRPC, and actions are sent back through the same interface. Inference runs on an external desktop equipped with an Intel i7 CPU, connected to the robot via Ethernet. Under this setup, the policy operates with 50~Hz as a lower bound and end-to-end latency of 2--5,ms.
    
    
    
    % spot: https://arxiv.org/abs/2504.17857
    Spot does not have explicit binary contact switches in its rubber feet. Instead, standard pipelines (such as the Spot RL Researcher Kit \cite{miller2025highperformancereinforcementlearningspot}) reconstruct contact states physically:
    \[
    \text{Contact State} = \begin{cases}
    1 \text{ (Stance)} & \text{if } |\tau_{\text{knee}}| > 8.0\text{ Nm} \\
    0 \text{ (Swing)} & \text{if } |\tau_{\text{knee}}| \le 8.0\text{ Nm}
    \end{cases}
    \]
    Because the knee joint torque ($\tau_{\text{knee}}$) is directly proportional to the vertical contact force $F_z$ via the leg Jacobian, thresholding the knee torque provides a robust, physics-grounded contact sensor.
    
    The policy is
      evaluated without command resampling under a scripted sagittal velocity profile:
      \[
      v_{\mathrm{cmd},x}(t) =
      \begin{cases}
      0.0~\mathrm{m/s}, & \text{stance phase},\\
      +0.5~\mathrm{m/s}, & \text{forward walking phase},\\
      -0.5~\mathrm{m/s}, & \text{backward walking phase}.
      \end{cases}
      \]
      The lateral and yaw commands are held at zero throughout the rollout,
      \[
      v_{\mathrm{cmd},y}(t)=0,\qquad \omega_{\mathrm{cmd},z}(t)=0.
      \]
    
      We use the same phase convention for visualization and downstream analysis as in the real-robot
      experiments. Timesteps with
      \[
      |v_{\mathrm{cmd},x}| \leq 0.1~\mathrm{m/s}
      \]
      are labeled as standing, timesteps with
      \[
      v_{\mathrm{cmd},x} > 0.1~\mathrm{m/s}
      \]
      as forward walking, and timesteps with
      \[
      v_{\mathrm{cmd},x} < -0.1~\mathrm{m/s}
      \]
      as backward walking.
    
    During each rollout, we log the commanded velocity, measured base velocity, projected gravity, joint
    positions, joint velocities, joint torques, foot contact states, foot heights, and phase identifiers. These
    trajectories are used to produce the visualizations and to compute phase-conditioned locomotion
    metrics such as velocity tracking, torso stability, cost of transport, and swing/stance gait statistics.
    
    We deployed 10 policy configurations recording 81,313 steps of high-resolution telemetry logged at 50\,Hz and isolating 193 steady-state forward gait strides. Tight 95\% bootstrap confidence intervals confirm that our architectural scaling advantages transfer robustly to hardware. 
    
    Under steady-state forward locomotion, the 8.45M parameter \text{SimBa-XXL} policy achieves a velocity tracking RMSE of $0.066\text{ m/s}$ (95\% CI: $[0.064, 0.067]$), outperforming the collapsed 1.89M \text{MLP-XXL} baseline ($0.176\text{ m/s}$, 95\% CI: $[0.086, 0.265]$) by 62.7\%. Furthermore, \text{SimBa-XXL} successfully mitigates joint-level jitter, restricting high-frequency ratio (HFR) to $0.64\%$ (95\% CI: $[0.61\%, 0.66\%]$) compared to $3.28\%$ (95\% CI: $[0.56\%, 6.00\%]$) for \text{MLP-XXL}, which exhibits severe physical leg chattering. This results could be understood as the lower-bound in efficiency and latency across all tested configurations. 
    
    
    
    \subsection{Training Details}
    
    Our experimental setup closely follows the Isaac Lab defaults, with specific modifications to improve simulation-to-real transfer regarding style, posture, and stability. The default locomotion training environment uses flat-plane terrain; while a rough terrain generator is present in the configuration file, it remains disabled in the baseline setup. The simulation executes at $200\,\text{Hz}$, while the policy control loop operates at $50\,\text{Hz}$. Each training episode has a maximum duration of $20\,\text{s}$ and terminates early if a timeout occurs or if any illegal contact involving the robot's main body or leg links is detected.
    
    In addition to the reward tuning detailed in the following section, we apply a symmetry-based data augmentation strategy to ensure sample efficiency and preserve real hardware. With this setup, each collected transition is mirrored along the robot's sagittal plane via a left--right mapping of observations and actions~\cite{rudin2022learning}, effectively doubling the usable batch size without requiring additional simulation time. This regularizes the policy, helping prevent overfitting or reward-hacking behaviors whose minor physical misalignments could potentially damage the hardware platform. 
    
    Furthermore, we designed an environmental curriculum spanning three registered environments. Progressing through these variants introduces an intentional weight curriculum that scales up selected penalty terms, most notably the base-orientation and contact-force penalties.
    
    Observations are not dynamically normalized during training in the standard \texttt{rsl\_rl} sense. Instead, normalization bounds are fixed based on prior empirical knowledge of the expected physical observation ranges. The complete set of architectural and algorithmic hyperparameters is reported in Table~\ref{tab:ppo_params}.
    
    \begin{table}[h]
    \centering
    \caption{Network architecture and PPO hyperparameters.}
    \label{tab:ppo_params}
    \ra{1.3}
    \begin{tabular}{lll}
    \hline
    \textbf{Category} & \textbf{Parameter} & \textbf{Value} \\
    \hline
    \multirow{3}{*}{Rollout}
      & Steps per environment            & $24$ \\
      & Parallel environments            & $4{,}096$ \\
      & Buffer size                      & ${\approx}\,49{,}152$ \\
    \hline
    \multirow{8}{*}{PPO}
      & Clipping parameter $\epsilon$   & $0.2$ \\
      & Value loss coefficient          & $1.0$ \\
      & Entropy coefficient             & $0.005$ \\
      & Learning rate schedule          & Adaptive \\
      & Target KL divergence            & $0.01$ \\
      & Learning epochs per iteration   & $5$ \\
      & Mini-batches per epoch          & $4$ \\
      & Max.\ gradient norm             & $1.0$ \\
    \hline
    \multirow{2}{*}{GAE}
      & Discount factor $\gamma$        & $0.99$ \\
      & GAE parameter $\lambda$         & $0.95$ \\
    \hline
    \end{tabular}
    \end{table}
    
    \paragraph{Reward Function}
    \label{sec:reward}
    
    The total reward $\mathcal{R}$ received at each timestep is a weighted sum of individual reward terms $r_i$, each scaled by a coefficient $w_i$:
    \begin{equation}
        \mathcal{R} = \sum_{i} w_i \, r_i.
        \label{eq:total_reward}
    \end{equation}
    
    The reward structure is designed to optimize stable, command-driven locomotion and mechanical efficiency while mitigating structural stress and unnatural postures. Crucially, the objective optimizes purely for locomotion tracking performance and explicitly excludes any arm reachability indices, end-effector trajectory tracking, or force-position manipulation targets. Each constituent term is detailed below.
    
    \textbf{Base Linear Velocity Tracking:} Rewards the agent for tracking commanded linear velocities along the $x$ and $y$ axes using an exponential kernel, with an additional scaling factor that increases the reward magnitude for higher commanded speeds:
    \begin{equation}
        r_{\text{lin\_vel}} = \exp\!\left(-\frac{\|\mathbf{v}_{xy}^{\text{cmd}} - \mathbf{v}_{xy}^{\text{base}}\|_2}{\sigma_{\text{lin}}}\right) \cdot \max\!\left(1,\; 1 + \gamma\bigl(\|\mathbf{v}_{xy}^{\text{cmd}}\|_2 - v_{\text{ramp}}\bigr)\right),
        \label{eq:lin_vel}
    \end{equation}
    where $\mathbf{v}_{xy}^{\text{cmd}}$ is the commanded planar velocity, $\mathbf{v}_{xy}^{\text{base}}$ is the robot's measured base planar velocity in the body frame, $\sigma_{\text{lin}}$ is the exponential kernel width, $v_{\text{ramp}}$ is the velocity threshold above which the scaling activates, and $\gamma$ is the ramp rate. This term has weight $w = 5.0$.
    
    \textbf{Base Angular Velocity Tracking:} Rewards yaw rate tracking. The first uses a wider standard deviation for general tracking, and the second (finer) uses a narrower standard deviation for high-precision tracking:
    \begin{equation}
    r_{\text{ang\_vel}} = \exp\!\left(-\frac{|\omega_z^{\text{cmd}} - \omega_z^{\text{base}}|}{\sigma_{\text{ang}}}\right),
    \label{eq:ang_vel}
\end{equation}
where $\omega_z^{\text{cmd}}$ is the commanded yaw rate and $\omega_z^{\text{base}}$ is the measured base yaw rate. Both terms carry weight $w = 5.0$, with different values of $\sigma_{\text{ang}}$.

\textbf{Gait Reward:} Enforces a trotting gait by synchronizing diagonal foot pairs (FL/HR and FR/HL). It is composed of two synchronization sub-rewards and four anti-synchronization sub-rewards:
\begin{equation}
    r_{\text{gait}} = R_{\text{sync}} \cdot R_{\text{async}},
    \label{eq:gait}
\end{equation}
where the synchronization reward for a pair $(f_0, f_1)$ is:
\begin{equation}
    R_{\text{sync}}(f_0, f_1) = \exp\!\left(-\frac{\text{clip}\bigl((t_{\text{air},f_0} - t_{\text{air},f_1})^2,\, \epsilon^2\bigr) + \text{clip}\bigl((t_{\text{con},f_0} - t_{\text{con},f_1})^2,\, \epsilon^2\bigr)}{\sigma_{\text{gait}}}\right),
    \label{eq:sync}
\end{equation}
and the anti-synchronization reward for an asynchronous pair $(f_0, f_1)$ is:
\begin{equation}
    R_{\text{async}}(f_0, f_1) = \exp\!\left(-\frac{\text{clip}\bigl((t_{\text{air},f_0} - t_{\text{con},f_1})^2,\, \epsilon^2\bigr) + \text{clip}\bigl((t_{\text{con},f_0} - t_{\text{air},f_1})^2,\, \epsilon^2\bigr)}{\sigma_{\text{gait}}}\right),
    \label{eq:async}
\end{equation}
where $t_{\text{air},f}$ and $t_{\text{con},f}$ are the current air time and contact time of foot $f$, $\epsilon$ is the maximum clipping error, and $\sigma_{\text{gait}}$ is the kernel width. The full gait reward is:
\begin{equation}
    r_{\text{gait}} = R_{\text{sync}}^{(0)} \cdot R_{\text{sync}}^{(1)} \cdot \prod_{k=0}^{3} R_{\text{async}}^{(k)}.
\end{equation}
This term is only applied when either the commanded velocity is nonzero or the body's planar speed exceeds a threshold $v_{\text{thr}}$. It has weight $w = 10.0$.

\textbf{Foot Clearance Reward:} Incentivizes the swinging feet to reach a target height $h^*$ above the ground, weighted by the foot's planar velocity to avoid rewarding stationary feet:
\begin{equation}
    r_{\text{clearance}} = \exp\!\left(-\frac{1}{\sigma_c}\sum_{f \in \mathcal{F}} \bigl(z_f - h^*\bigr)^2 \cdot \tanh\!\bigl(\alpha \|\mathbf{v}_{xy,f}\|_2\bigr)\right),
    \label{eq:clearance}
\end{equation}
where $z_f$ is the world-frame height of foot $f$, $h^* = 0.1$\,m is the target swing height, $\alpha$ is the tanh scaling factor, $\sigma_c$ is the kernel width, and $\mathcal{F}$ is the set of feet. This term has weight $w = 0.5$.

\textbf{Action Smoothness Penalty:} Discourages large instantaneous changes in the policy's output action vector $\mathbf{a}$:
\begin{equation}
    p_{\text{smooth}} = \|\mathbf{a}_t - \mathbf{a}_{t-1}\|_2,
    \label{eq:smoothness}
\end{equation}
where $\mathbf{a}_t$ and $\mathbf{a}_{t-1}$ are the current and previous network actions. Weight: $w = -1.0$.

\textbf{Air Time Variance Penalty:} Discourages asymmetric foot timing by penalizing the variance in last air and contact times across feet:
\begin{equation}
    p_{\text{air\_var}} = \mathrm{Var}\!\left(\text{clip}(\mathbf{t}_{\text{air}},\, 0.5)\right) + \mathrm{Var}\!\left(\text{clip}(\mathbf{t}_{\text{con}},\, 0.5)\right),
    \label{eq:air_var}
\end{equation}
where $\mathbf{t}_{\text{air}}$ and $\mathbf{t}_{\text{con}}$ are vectors of the last air and contact times for all feet. Weight: $w = -1.0$.

\textbf{Base Motion Penalty:} Discourages excessive vertical linear and roll/pitch angular acceleration of the base:
\begin{equation}
    p_{\text{motion}} = 0.8\,\dot{v}_z^2 + 0.2\,\bigl(|\dot{\omega}_x| + |\dot{\omega}_y|\bigr),
    \label{eq:base_motion}
\end{equation}
where $\dot{v}_z$ is the base vertical linear velocity and $\dot{\omega}_x,\,\dot{\omega}_y$ are the base roll and pitch angular velocities. Weight: $w = -2.0$.

\textbf{Base Orientation Penalty:} Discourages tilting of the robot's base by measuring the deviation from the gravity vector:
\begin{equation}
    p_{\text{orient}} = \|\mathbf{g}_{\perp}\|_2,
    \label{eq:orient}
\end{equation}
where $\mathbf{g}_{\perp} \in \mathbb{R}^2$ are the $x$- and $y$-components of the projected gravity vector in the base frame (which are zero when the base is level). Weight: $w = -3.0$.

\textbf{Foot Slip Penalty:} Discourages feet from sliding while in ground contact:
\begin{equation}
    p_{\text{slip}} = \sum_{f \in \mathcal{F}} \mathbb{1}[f \text{ in contact}] \cdot \|\mathbf{v}_{xy,f}\|_2,
    \label{eq:slip}
\end{equation}
where contact is determined by comparing the net contact force magnitude against a threshold. Weight: $w = -0.5$.

\textbf{Joint Position Penalty:} Encourages joints to remain near their nominal configuration. When the robot is at a standstill (low command and low body velocity), the penalty is scaled up by a factor $\kappa$:
\begin{equation}
    p_{\text{jpos}} =
    \begin{cases}
        \|\mathbf{q}_{\text{leg}} - \mathbf{q}_{0,\text{leg}}\|_2 & \text{if } \|\mathbf{v}^{\text{cmd}}\| > 0 \text{ or } v_{\text{body}} > v_{\text{thr}}, \\
        \kappa\,\|\mathbf{q}_{\text{leg}} - \mathbf{q}_{0,\text{leg}}\|_2 & \text{otherwise},
    \end{cases}
    \label{eq:jpos}
\end{equation}
where $\mathbf{q}_{\text{leg}}$ is the current joint position vector for the legs and $\mathbf{q}_{0,\text{leg}}$ is their default nominal configuration. Weight: $w = -0.7$.

\textbf{Joint Velocity, Acceleration, and Torque Penalties:} Reduces mechanical stress and promotes smooth motion, joint velocities, accelerations, and torques are penalized by their $\ell_2$ norms:
\begin{align}
    p_{\text{jvel}}  &= \|\dot{\mathbf{q}}\|_2, \quad w = -0.01, \label{eq:jvel} \\
    p_{\text{jacc}}  &= \|\ddot{\mathbf{q}}\|_2, \quad w = -10^{-4}, \label{eq:jacc} \\
    p_{\text{jtor}}  &= \|\boldsymbol{\tau}\|_2,  \quad w = -5 \times 10^{-4}, \label{eq:jtor}
\end{align}
where $\dot{\mathbf{q}}$, $\ddot{\mathbf{q}}$, and $\boldsymbol{\tau}$ are the joint velocity, acceleration, and applied torque vectors across the active joints.

\textbf{Contact Force Penalty:} To actively protect structural elements from excessive impact loads during fast transitions or falls, vertical ground contact forces exceeding a safe nominal threshold are penalized:
\begin{equation}
    p_{\text{contact}} = \sum_{f \in \mathcal{F}} \max\bigl(0, \|\mathbf{F}_{f}\|_2 - F_{\text{max}}\bigr),
    \label{eq:contact}
\end{equation}
where $\mathbf{F}_{f}$ represents the measured contact force vector at foot $f$ and $F_{\text{max}}$ denotes the safety limit. This term is heavily scaled within environmental curriculum stages.

\textbf{Reward Summary}

Table~\ref{tab:reward_terms} summarizes all reward and penalty terms with their respective weights.

\begin{table}[h!]
\centering
\caption{Reward and penalty terms of the locomotion training objective.}
\label{tab:reward_terms}
\renewcommand{\arraystretch}{1.3}
\begin{tabular}{llcl}
\hline
\textbf{Term} & \textbf{Equation} & \textbf{Weight} & \textbf{Description} \\
\hline
Base linear velocity    & Eq.~\eqref{eq:lin_vel}     & $+5.0$              & XY velocity tracking \\
Base angular velocity   & Eq.~\eqref{eq:ang_vel}     & $+5.0$              & Yaw rate tracking  \\
Base angular vel. (fine)& Eq.~\eqref{eq:ang_vel}     & $+5.0$              & Yaw rate tracking (high precision) \\
Gait                    & Eq.~\eqref{eq:gait}        & $+10.0$             & Enforces trotting via foot sync \\
Foot clearance          & Eq.~\eqref{eq:clearance}   & $+0.5$              & Encourages 0.1\,m swing height \\
Action smoothness       & Eq.~\eqref{eq:smoothness}  & $-1.0$              & Penalizes sudden action changes \\
Air time variance       & Eq.~\eqref{eq:air_var}     & $-1.0$              & Penalizes uneven foot timing \\
Base motion             & Eq.~\eqref{eq:base_motion} & $-2.0$              & Penalizes base undesired motion \\
Base orientation        & Eq.~\eqref{eq:orient}      & $-3.0$              & Penalizes base tilt \\
Foot slip               & Eq.~\eqref{eq:slip}        & $-0.5$              & Penalizes sliding feet \\
Joint position          & Eq.~\eqref{eq:jpos}        & $-0.7$              & Encourages nominal leg joint configuration \\
Joint velocity          & Eq.~\eqref{eq:jvel}        & $-0.01$             & Penalizes high joint speeds \\
Joint acceleration      & Eq.~\eqref{eq:jacc}        & $-10^{-4}$          & Penalizes high joint accelerations \\
Joint torques           & Eq.~\eqref{eq:jtor}        & $-5{\times}10^{-4}$ & Penalizes high joint torques \\
Contact force           & Eq.~\eqref{eq:contact}     & $-10^{-3}$          & Penalizes excessive foot impact forces \\
\hline
\end{tabular}
\end{table}

%------------------------------------------------------------------------------
\paragraph{Domain Randomization}
\label{sec:domain_rand}

To narrow the sim-to-real gap, several domain randomization schemes are applied at different phases of the simulation runtime: at startup initialization, at individual episode resets, and periodically inside active environments.

At startup, four properties alter the structural dynamics of the robot asset and terrain interface. The ground surface friction coefficient is randomized, and the physical masses of the robot base, the attached arm, and the leg links are perturbed. Base and arm mass updates receive additive deviations, while leg segments undergo multiplicative scaling.

At each episode reset, three additional operations diversify the initial boundary state conditions. Random impulsive forces and torques are briefly applied to the robot base, the initial base yaw heading and planar coordinate placement are offset, and initial joint configurations are initialized with random noise distributed around their default nominal values.

Finally, while an episode is active, external push disturbances are periodically applied to the robot base at intervals ranging between 7 and 10 seconds. These force/torque perturbations and external pushes are fully phased into training using curriculum terms as policy optimization advances. Table~\ref{tab:randomization} details the complete parameter sets.

\begin{table}[h!]
\centering
\caption{Domain randomization events applied during training.}
\label{tab:randomization}
\renewcommand{\arraystretch}{1.3}
\begin{tabular}{lll}
\hline
\textbf{Event} & \textbf{Stage} & \textbf{Range / Parameter} \\
\hline
Ground Friction         & Startup  & Friction $\in [0.3, 1.0]$ \\
Base Mass Perturbation  & Startup  & $\Delta m \in [-2.5, 2.5]$\,kg \\
Arm Mass Perturbation   & Startup  & $\Delta m \in [-0.5, 0.5]$\,kg \\
Leg Mass Scaling        & Startup  & Scale $\in [0.8\times, 1.5\times]$ \\
Impulsive Wrench        & Reset    & $F = 10$\,N, $\tau = 2$\,Nm \\
Base Pose Reset         & Reset    & Yaw $\in [-\pi, \pi]$, Pos $\in [-0.5, 0.5]$\,m \\
Joint Initialization    & Reset    & Sampled around nominal configuration \\
Base Velocity Push      & Interval & Every 7--10\,s (via curriculum) \\
\hline
\end{tabular}
\end{table}


\paragraph{Observation Space}
\label{sec:observations}

At each control step, the policy receives a concatenated observation vector $\mathbf{o}_t \in \mathbb{R}^{65}$. To regularize the policy against sensor delays and estimation errors, observation corruption via additive zero-mean Gaussian noise is enabled throughout training. The full observation vector decomposes into the following modalities:

\begin{itemize}
    \item \textbf{Base state}: Linear velocity $\mathbf{v}^{\text{base}} \in \mathbb{R}^3$, angular velocity $\boldsymbol{\omega}^{\text{base}} \in \mathbb{R}^3$, and the gravity vector projected into the body frame $\mathbf{g}_b \in \mathbb{R}^3$.
    \item \textbf{Command}: Planar base velocity targets $(v_x^{\text{cmd}}, v_y^{\text{cmd}}, \omega_z^{\text{cmd}}) \in \mathbb{R}^3$, commanded base height target $h^{\text{cmd}} \in \mathbb{R}^1$, and target base orientation components (roll and pitch) $\boldsymbol{\theta}^{\text{cmd}} \in \mathbb{R}^2$.
    \item \textbf{Joint state}: Relative joint positions $\mathbf{q} - \mathbf{q}_0 \in \mathbb{R}^{19}$ and joint velocities $\dot{\mathbf{q}} \in \mathbb{R}^{19}$, which map across the 12 leg joints and 7 arm joints.
    \item \textbf{History}: The previous execution step's 12-dimensional policy action command $\mathbf{a}_{t-1} \in \mathbb{R}^{12}$.
        \end{itemize}

The specific multi-command environment generates target updates every $10\,\text{s}$. Forward velocity is sampled within $[-1.0, 1.0]\,\text{m/s}$, lateral velocity within $[-0.5, 0.5]\,\text{m/s}$, yaw rate within $[-1.0, 1.0]\,\text{rad/s}$, and heading angle targets within $[-\pi, \pi]\,\text{rad}$, with explicit heading-tracking mode enabled for exactly half of the active environments. Base orientation commands sample roll and pitch ranges within $[-0.5, 0.5]\,\text{rad}$, enforcing a level flat-orientation constraint ($0\,\text{rad}$) for $40\%$ of the parallel tracks. Base height targets are uniformly sampled within the range $[0.5, 0.7]\,\text{m}$.

\paragraph{Action Space}
\label{sec:actions}

The policy action space $\mathbf{a}_t \in \mathbb{R}^{12}$ is defined as a $12$-dimensional vector corresponding to joint-position targets for the active Spot leg joints. These targets are scaled by a factor of $0.2$ and added as angular displacement deltas around the nominal leg joint offsets $\mathbf{q}_{0,\text{leg}}$. Although the simulated physical asset represents the full Spot quadruped complete with its attached arm system, the locomotion policy does not command arm motion. Instead, the 7 arm joints are maintained at a rigid, fixed default reset configuration using a constant joint-position control loop with zero action dimension, ensuring they do not consume policy outputs or modify the action space.
